# Supplementary material for: Asynchronous and Load-Balanced Union-Find for Distributed and Parallel Scientific Data Visualization and Analysis
Source: arXiv:2003.02351 source file (2021-04-13)
Supplement: Supplementary file 1 [file 8_appendix.tex]

\section{Transitions between Processes' States in Asynchronous Termination Detection}
We summarize the transitions between processes' states for the asynchronous termination detection mentioned in \cite{dathathri2019gluon}. 
\begin{enumerate}
  \item \textit{Active}: 
    A process starts from an \textit{active} state. As long as the process updates its data, sends or receives any messages about the data update, no matter the current state of the process is, the state of the process becomes \textit{active}. 
  \item \textit{Idle: }
    An \textit{active} process changes its state to \textit{idle} when the process has no local computation work to do. 
  \item \textit{Ready-to-terminate: }
    If a process becomes \textit{idle} at its $n$th iteration and remains in \textit{idle} after, that process becomes \textit{ready-to-terminate} when the process receives the state messages from all other processes at the $(n+1)$th iteration; intuitively, \textit{ready-to-terminate} indicates the process finishes all work and receives all data update messages until the $n$th iteration.  
  \item \textit{Terminate: }
    If a process becomes \textit{ready-to-terminate} at its $n$th iteration and remains in \textit{ready-to-terminate} after, that process becomes \textit{terminate} when the process receives the state messages from all other processes at an $m$th ($m \geq n$) iteration and knows all processes are in the states of \textit{ready-to-terminate} at the $m$th iteration. When a process reaches the \textit{terminate} state, the process knows all other processes have finished work, and hence, the distributed iterative algorithm can terminate. 
\end{enumerate}

\section{Effect of Varying Sizes of Data Blocks}
% {Benchmark on $256^3$ Synthetic Data}
We include additional studies, which show that the performance improvements (i.e., speedups) of our algorithm over the baseline are consistent with varying sizes of data blocks in both strong and weak scaling studies.

\begin{figure}[htb]
\centering
\includegraphics[width=\linewidth]{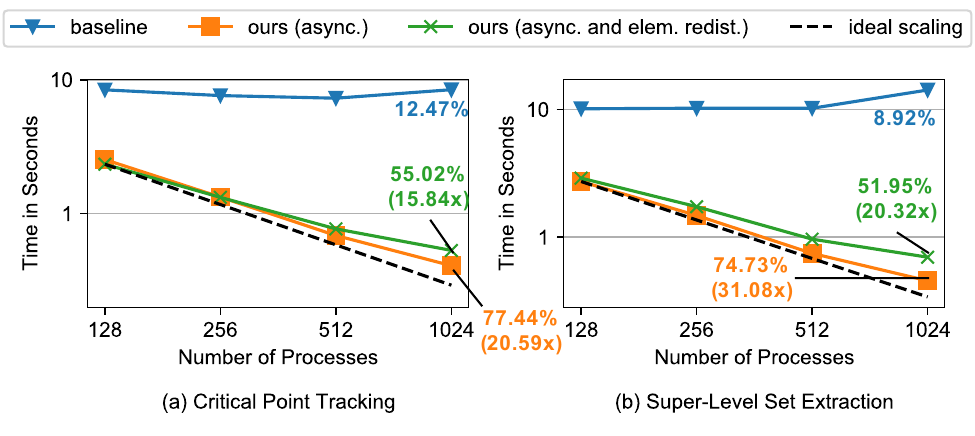}

%   \vspace{-1em}
  \caption{Strong scaling of distributed union-find on $256^3$ synthetic data using $128$ to $1,024$ processes for (a) tracking critical points and (b) extracting super-level sets. Both axes are log scales. 
  }
%   \vspace{-1.5em}
  
  \label{fig:sync_vs_async_256}
\end{figure}

\subsection{Strong Scaling Study}
With respect to the strong scaling, our algorithms have consistent performance improvements (i.e., speedups) over the baseline when the sizes of data blocks vary by comparing Fig.~4 using $1,024^3$ data and Fig.~\ref{fig:sync_vs_async_256} using $256^3$ data. 

We included an additional strong scaling study for $256^3$ synthetic data in Fig.~\ref{fig:sync_vs_async_256}. 
Compared with the baseline, our asynchronous algorithm \textit{without} the element redistribution attains $20.59$x speedup in the critical point tracking benchmark and $31.08$x speedup in the super-level set extraction benchmark when $1,024$ processes are used; our asynchronous algorithm \textit{with} the element redistribution attains $15.84$x and $20.32$x speedup in the two benchmarks.

% \remark{Our algorithm with the element redistribution becomes relatively slower than the case without the redistribution when smaller data block sizes are used for the synthetic data. }

\begin{figure}[htb]
\centering
\includegraphics[width=\linewidth]{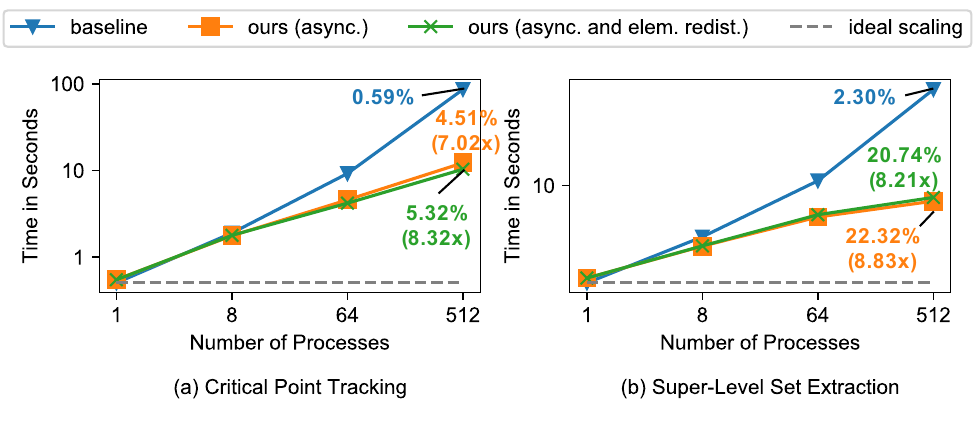}

%   \vspace{-1em}
  \caption{Weak scaling of distributed union-find on synthetic data. 
  Each process is assigned with a $64^3$ mesh grid with a constant feature density. 
  We use four combinations of data resolutions and process counts: $64^3$ with $1$ process, $128^3$ with $8$ processes, $256^3$ with $64$ processes, and $512^3$ with $512$ processes. Both axes are log scales. }
%   \vspace{-1.5em}
  
  \label{fig:weak_scaling_64}
\end{figure}

\subsection{Weak Scaling Study}
With respect to the weak scaling, our algorithms also obtain consistent performance improvements over the baseline when varying the sizes of data blocks by comparing Fig.~\ref{fig:sync_vs_async_256} using $64^3$ mesh grid per process and Fig.~7 using $32^3$ grid per process. 

\remark{We included an additional weak scaling study with a $64^3$ grid per process in Fig.~\ref{fig:weak_scaling_64}. }
Compared with the baseline, our asynchronous algorithm \textit{without} the element redistribution attains $7.02$x speedup in the critical point tracking benchmark and $8.83$x speedup in the super-level set extraction benchmark when $512$ processes are used; our asynchronous algorithm \textit{with} the element redistribution attains $8.32$x and $8.21$x speedup in the two benchmarks.

\begin{figure}[htb]
\centering
\includegraphics[width=\linewidth]{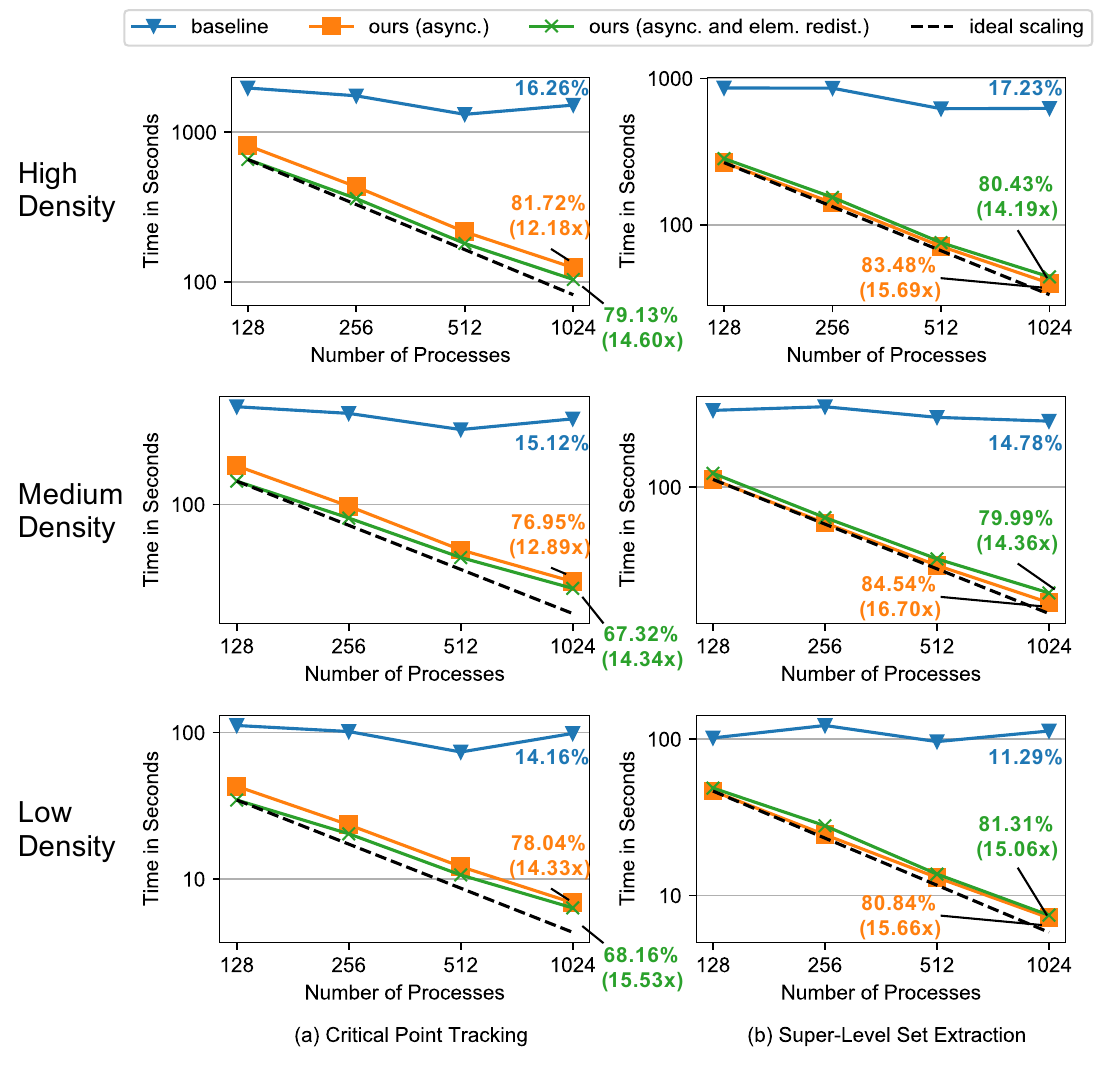}

%   \vspace{-1em}
  \caption{Strong scaling on $1,024^3$ synthetic data with three feature density levels: high, medium, and low density in three rows for (a) tracking critical points and (b) tracking super-level sets in two columns. }
%   \vspace{-1.5em}
  
  \label{fig:feature_densities}
\end{figure}

\section{Effect of Varying Feature Densities}

We evaluate the performance of the baseline approach and our distributed union-find algorithms when the feature density of the data varies in space and time. \remark{Results indicate the performance improvements of our algorithm over the baseline are consistent with varying feature densities. }

We test the methods on $1,024^3$ synthetic data with three levels of feature density: (1) low feature density, (2) medium feature density, and (3) high feature density; the data are generated by fixing the data resolution to be  $1,024^3$ and varying the number of features in space and time. 
For tracking critical points, the high feature density case has $161,338,942$ critical points in space and time, the medium-density one has $40,280,575$ critical points, and the low-density one has $10,066,949$ critical points. For tracking super-level sets, the high feature density case has $72,097,212$ extracted voxels, the medium-density one has $35,071,247$ voxels, and the low-density one has $17,309,120$ voxels.

The results are shown in Fig.~\ref{fig:feature_densities}. 
For critical point tracking, when using $1,024$ processes, 
% the baseline approach attains the strong scaling efficiency of $0.17\%$, $0.54\%$, and $1.27\%$ on the low, medium, and high feature density data, respectively. In contrast, our approach has $3.52\%$, $14.35\%$, and $26.75\%$ efficiency. 
compared with the baseline, our asynchronous algorithm \textit{without} the element redistribution achieves $12.18$x, $12.89$x, and $14.33$x speedup on the data with the three levels of feature density; our asynchronous algorithm \textit{with} the element redistribution achieves $14.60$x, $14.34$x, and $15.53$x speedup, respectively. 
For super-level set tracking, when using $1,024$ processes, 
% the baseline approach attains the strong scaling efficiency of $0.42\%$, $0.57\%$, and $0.66\%$ on the low, medium, and high feature density data. On the contrary, our method has $12.86\%$, $21.00\%$, and $25.47\%$ efficiency. 
compared with the baseline, our asynchronous algorithm \textit{without} the element redistribution achieves $15.69$x, $16.70$x, and $15.66$x speedup on the data of low, medium, and high feature density; our asynchronous algorithm \textit{with} the element redistribution achieves $14.19$x, $14.36$x, and $15.06$x speedup, respectively.

% We included a strong scaling study for $1,024^3$ synthetic data with varying numbers of features in Fig.~\ref{fig:feature_densities} of this cover letter and in the supplementary material of the revised paper due to the paper length limit. Fig.~\ref{fig:feature_densities} reveals that the speedups of our algorithm over the baseline for the $1,024^3$ case with different levels of feature densities are similar, indicating the performance improvements are consistent with varying numbers of features. 

% On average, our method gets $21.09$x speedup on critical point tracking and $31.96$x on super-level set tracking compared with the baseline approach. When increasing the feature density in space, the strong scaling efficiency of our method increases. The reasons are as follows. When there is a higher feature density in space, processes need more time to complete the local computation. Since we overlap local computation and communication, longer computational time can cover more communication overhead. Hence, we attain better strong scaling when the feature density of data is higher. 

% since the workload of different processes is unbalanced when making the barrier synchronization after finishing one round of computation, 
% ; that causes waste of computational resources. 
% In summary, we have two observations from the results in Fig.~\ref{fig:feature_densities}. First, by comparing with the baseline approach, the speedup of our method is stable for data with different feature densities. 

\section{Cost Breakdown of Feature Extraction and Tracking Framework}

% We measure our feature extraction and tracking pipeline's performance to track critical points on exploding wire data and track super-level sets on BOUT++ data. 
% As shown in Fig.~\ref{fig:scientific_data_pipeline}, when using $1,024$ processes, our feature tracking method attains $59.62\%$ strong scaling efficiency on the exploding wire data, and $3.03\%$ efficiency on the BOUT++ data. The scaling efficiency on the BOUT++ data is relatively low and explained by the time percentage breakdown below. 

% The time percentage breakdown in Fig.~\ref{fig:scientific_data_pipeline_breakdown} indicates the time percentages of different steps within the whole pipeline, 

% In Fig.~\ref{fig:breakdown_a}, 
% for the critical point tracking 

We included a cost breakdown of different stages of the feature extraction and tracking framework with respect to different counts of processes in Fig.~\ref{fig:scientific_data_pipeline_breakdown}. 
For the critical point tracking in exploding wire experimental data, the majority of the cost is the critical point detection. 
For the super-level set extraction in fusion plasm simulation data, as compared with other steps, the time of the distributed union-find based CCL shrinks as we use more processes, which shows that our distributed union-find algorithm has a good scaling. 
%  compared with other steps
% for the super-level set tracking
% A limitation on the BOUT++ data is that, in Fig.~\ref{fig:bout_breakdown_a}, the finalization step does not scale well and hampers the scaling of the whole pipeline in Fig.~\ref{fig:scientific_data_pipeline}b. The reason is that, to collect features and output trajectories, we need to gather distributed elements with the same identifiers to the same processes, which is based on \texttt{MPI\_Alltoall} operation; the \texttt{MPI\_Alltoall} operation is hard to scale well when each connected component has a large number of features. 

\begin{figure}[htb]
\centering
\includegraphics[width=\linewidth]{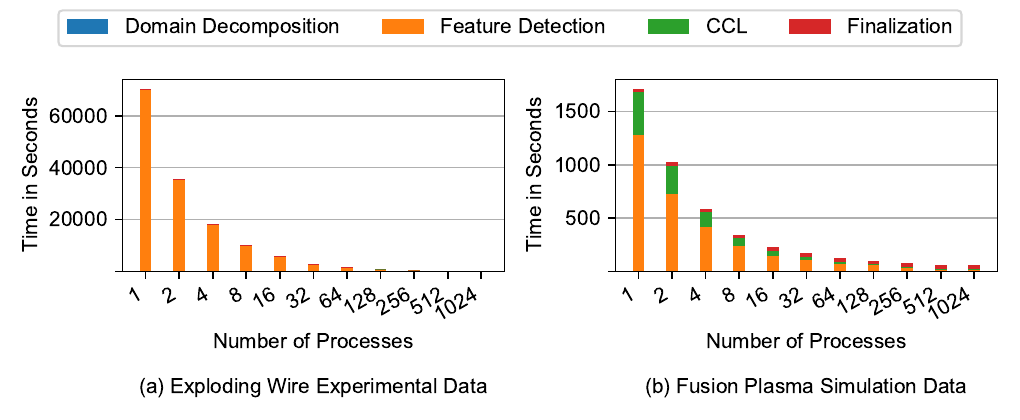}

%   \vspace{-1em}
  \caption{Breakdown of the time cost of different stages of the used feature extraction and tracking framework in two application datasets. The horizontal axis is a log scale. }
%   \vspace{-1.5em}
  
  \label{fig:scientific_data_pipeline_breakdown}
\end{figure}
